# Supplementary material for: Towards Optimal Robustness of Network Controllability: An Empirical Necessary Condition
Source: arXiv:1912.12416 source file (2020-09-01)
Supplement: Supplementary file 1 [file arXiv_si.pdf]

# Supplementary Information for the Paper "Towards Optimal Robustness of Network Controllability: An Empirical Necessary Condition"

Yang Lou[1], Lin Wang[2,3], Kim Fung Tsang[1], and Guanrong Chen [*] [†] [‡] [1]

[1]Department of Electrical Engineering, City University of Hong Kong, Hong Kong, China
[2]Department of Automation, Shanghai Jiao Tong University, Shanghai 200240, China
[3]Key Laboratory of System Control and Information Processing, Ministry of Education, Shanghai 200240, China

## 1 Optimal Topology

Figures S1, S2, and S3 show the optimal network instances of small-sized networks. The number of nodes $N$ and number of edges $M$ are shown in Table S1, together with the number of possible instances (PI), and the number of instances with optimal robustness of controllability (O).

Table S1: $N$ and $M$ represent the number of nodes and edges, respectively. PI represents the number of possible network instances with given $N$ and $M$. O represents the number of optimal robustness instances.

| $N$ | 4 | | | | | | | | 6 | | | | | | |
|---|---|---|---|---|---|---|---|---|---|---|---|---|---|---|---|
| $M$ | 4 | 5 | 6 | 7 | 8 | 9 | 10 | 11 | 6 | 24 | 25 | 26 | 27 | 28 | 29 |
| PI | 22 | 37 | 47 | 38 | 27 | 13 | 5 | 1 | 582 | 1043 | 288 | 76 | 17 | 5 | 1 |
| O | 1 | 1 | 2 | 1 | 1 | 2 | 2 | 1 | 1 | 2 | 4 | 5 | 4 | 2 | 1 |
| $N$ | 5 | | | | | | | | | | | | | | |
| $M$ | 5 | 6 | 7 | 8 | 9 | 10 | 11 | 12 | 13 | 14 | 15 | 16 | 17 | 18 | 19 |
| PI | 108 | 326 | 667 | 1127 | 1477 | 1665 | 1489 | 1154 | 707 | 379 | 154 | 61 | 16 | 5 | 1 |
| O | 1 | 1 | 2 | 2 | 1 | 1 | 1 | 2 | 2 | 1 | 1 | 3 | 3 | 2 | 1 |

[*]Corresponding author: G. Chen (eegchen@cityu.edu.hk).
E-mails: Y. Lou (felix.lou@my.cityu.edu.hk), K.F. Tsang (ee330015@cityu.edu.hk), L. Wang (wanglin@sjtu.edu.cn).

[†]Supplementary Information: Y. Lou, L. Wang, K.F. Tsang, and G. Chen, "Towards Optimal Robustness of Network Controllability: An Empirical Necessary Condition," *IEEE Transactions on Circuits and Systems I: Regular Papers*, 67(9): 3163–3174; doi:10.1109/TCSI.2020.2986215 (2020).

[‡]Source Code: `https://fylou.github.io/sourcecode.html`

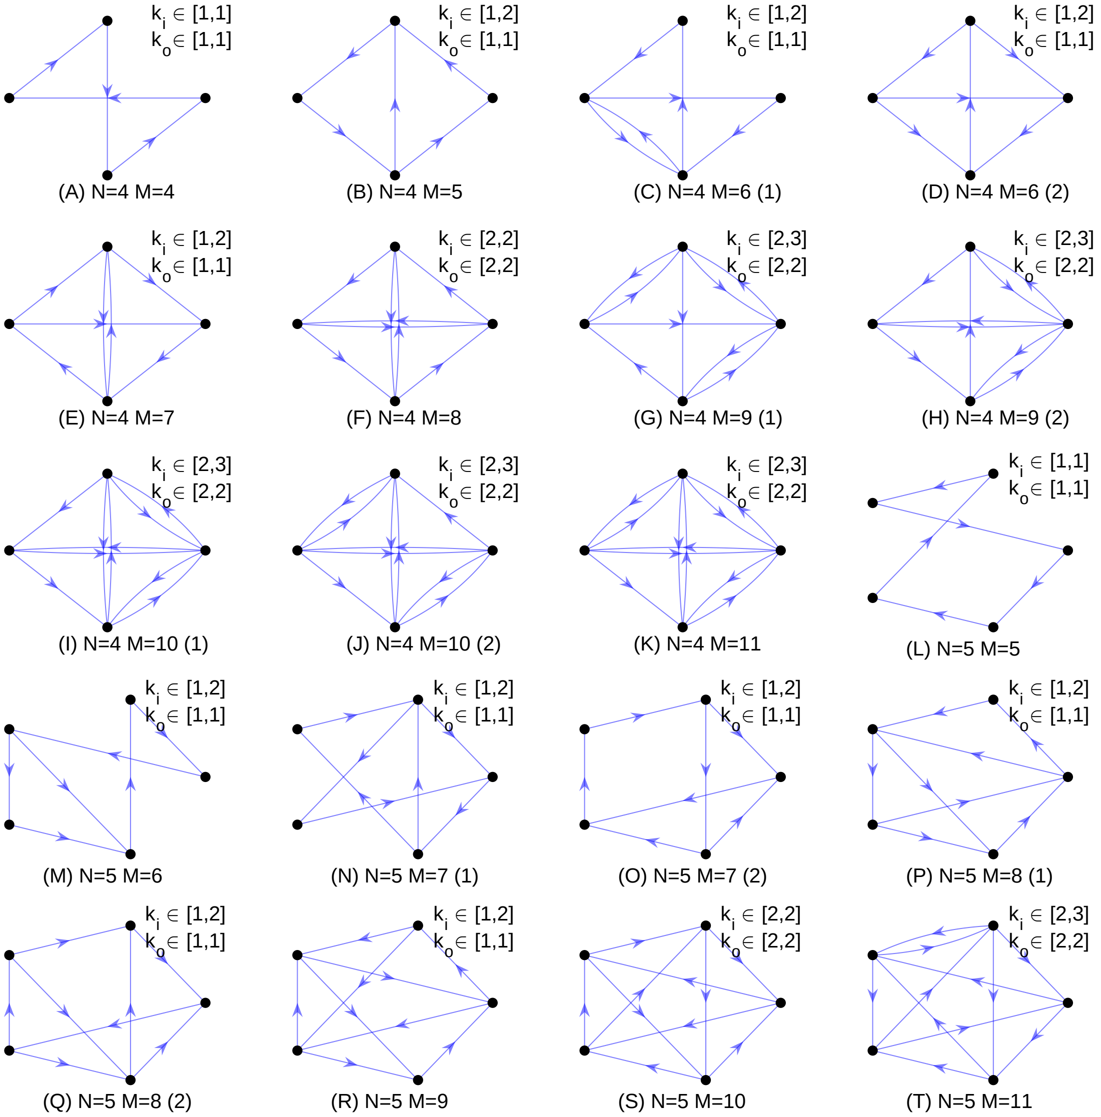


Figure S1: Optimal network topology of very small-sized networks (Part I).

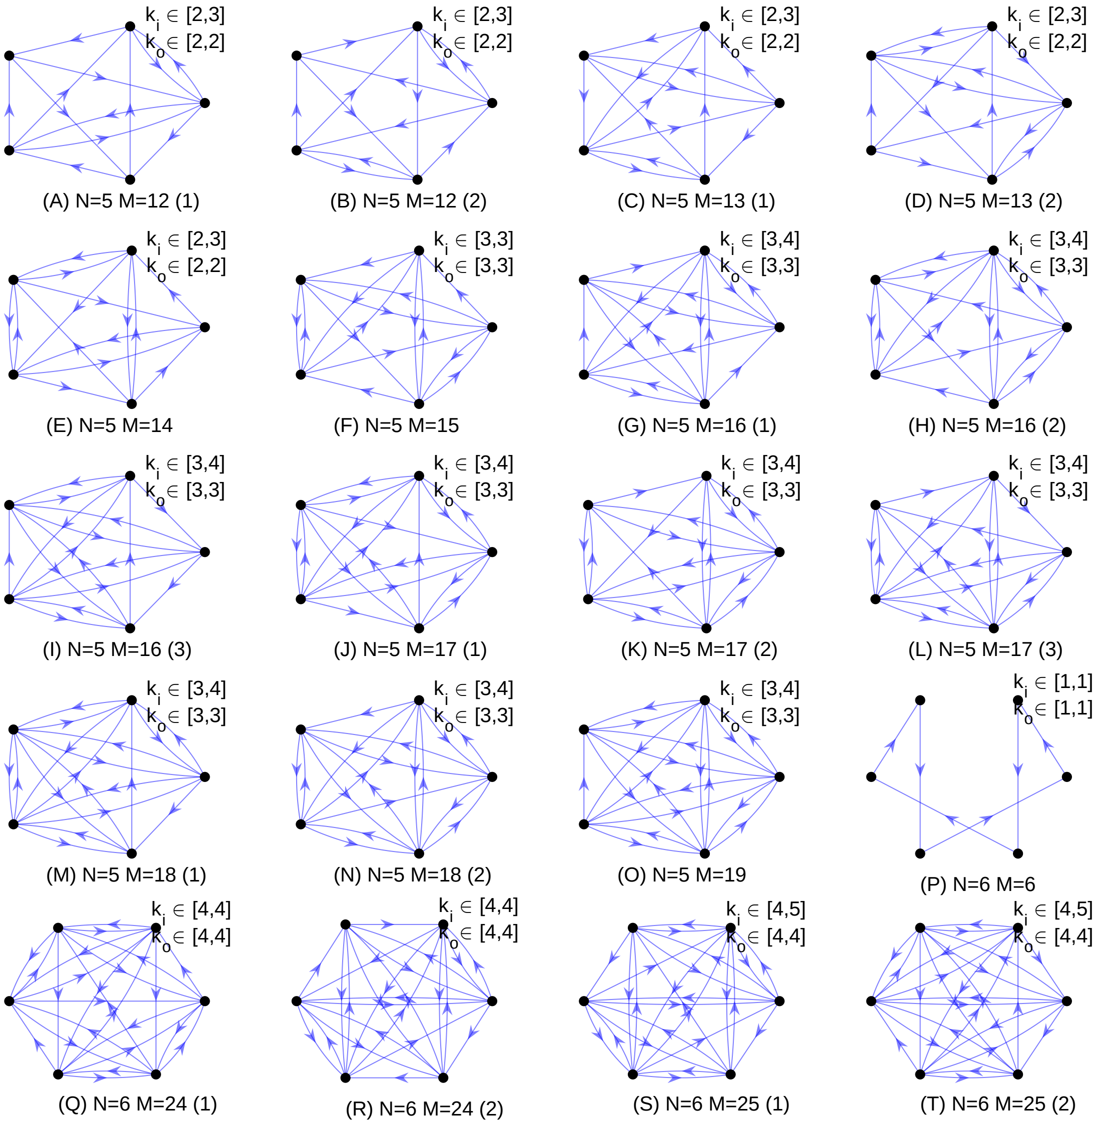


Figure S2: Optimal network topology of very small-sized networks (Part II).

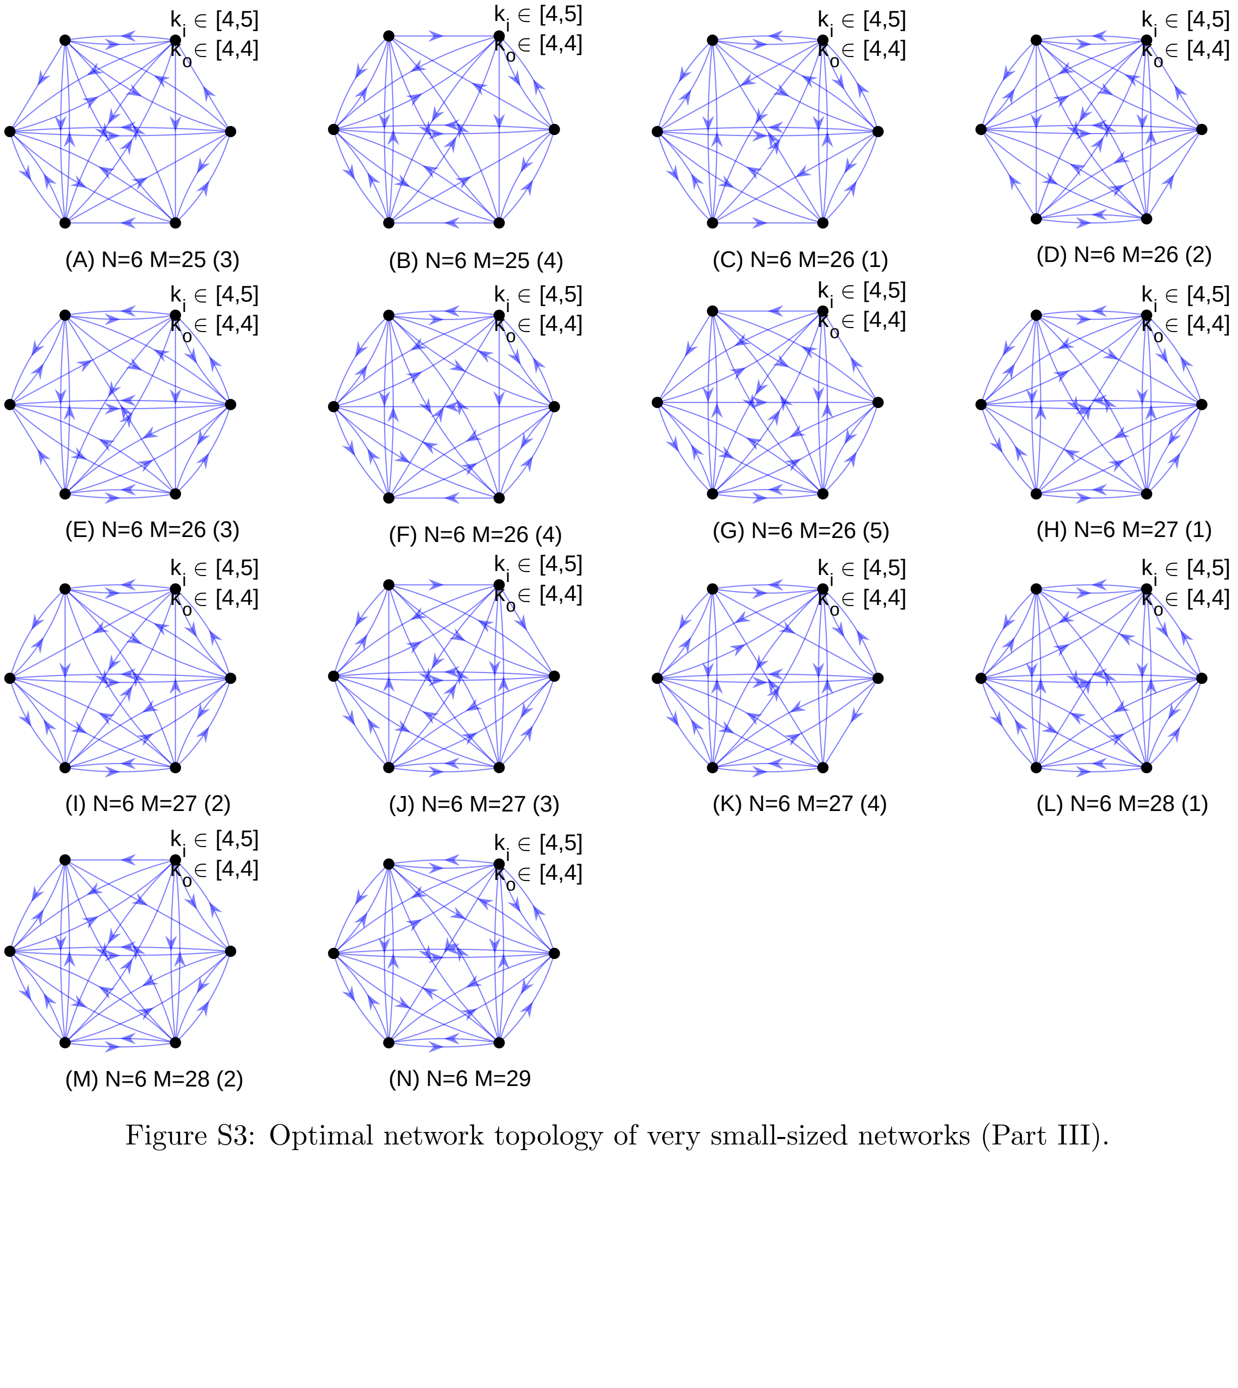


Figure S3: Optimal network topology of very small-sized networks (Part III).

## 2 Robustness of Exact Controllability

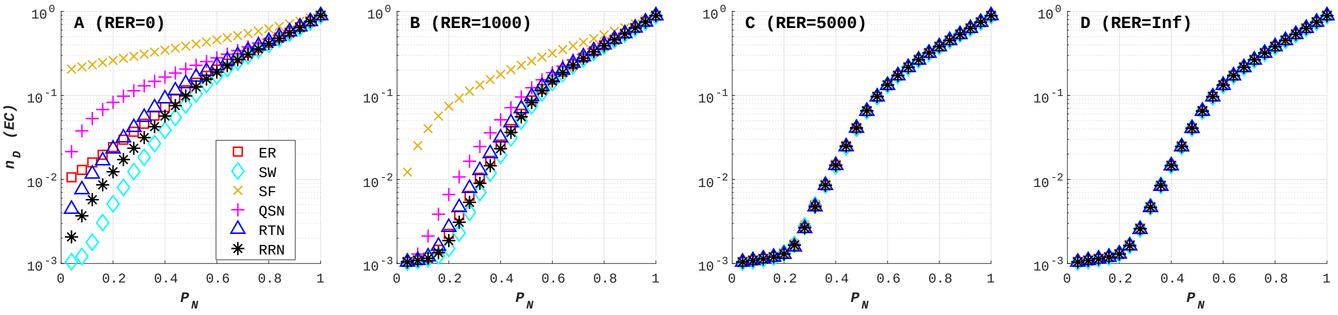


Figure S4: Robustness of *exact* controllability of the six networks: (A) without any rectification; (B) with 1000 RER operations; (C) with 5000 RER operations; (D) with RER operations until ENC is satisfied. $n_D$ represents density of control-nodes calculated in terms of exact controllability. $P_N$ represents the proportion of removed nodes.

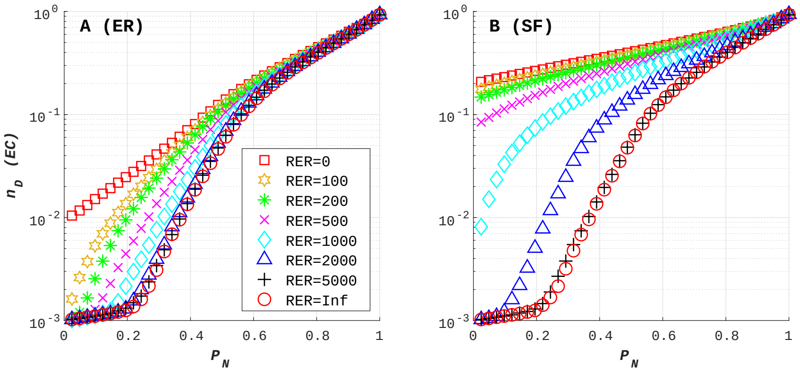


Figure S5: Robustness of *exact* controllability of (A) ER and (B) SF, when the number of RER varies from 0 to infinity. $n_D$ represents density of control-nodes; $P_N$ represents the proportion of removed nodes.

# 3 Average Out-degree $\langle k^{out} \rangle = \{3, 8\}$

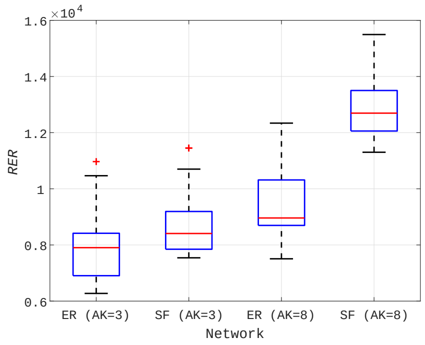


Figure S6: Number of RER operations to rectify a network to satisfy the ENC. The network configuration is $\langle k^{out} \rangle = 3$ and $\langle k^{out} \rangle = 8$; the number of repeated runs is 100.

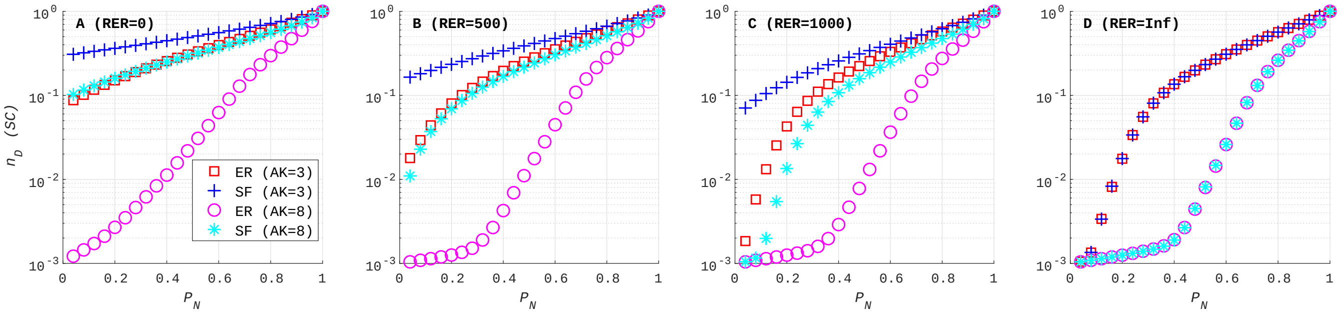


Figure S7: Robustness of *structural* controllability of the six networks: (A) without any rectification; (B) with 500 RER operations; (C) with 1000 RER operations; (D) with RER operations until ENC is satisfied. $n_D$ represents density of control-nodes; $P_N$ represents the proportion of removed nodes.

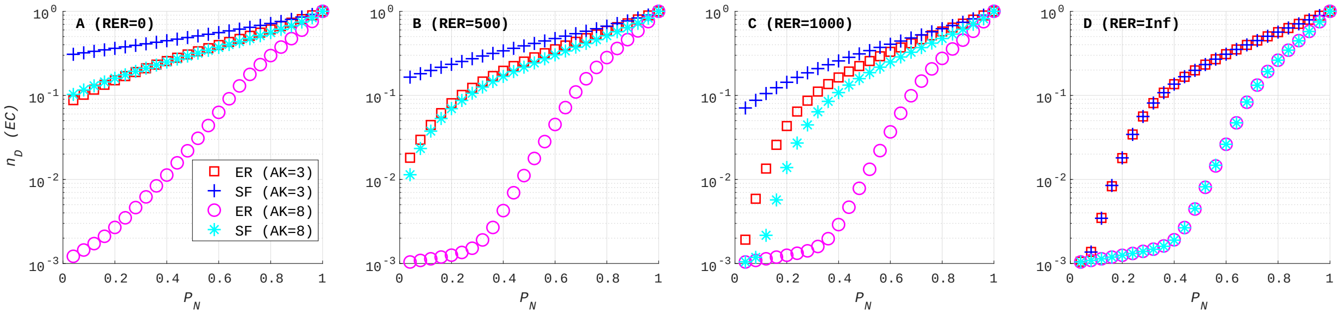


Figure S8: Robustness of *exact* controllability of the six networks: (A) without any rectification; (B) with 500 RER operations; (C) with 1000 RER operations; (D) with RER operations until ENC is satisfied. $n_D$ represents density of control-nodes; $P_N$ represents the proportion of removed nodes.

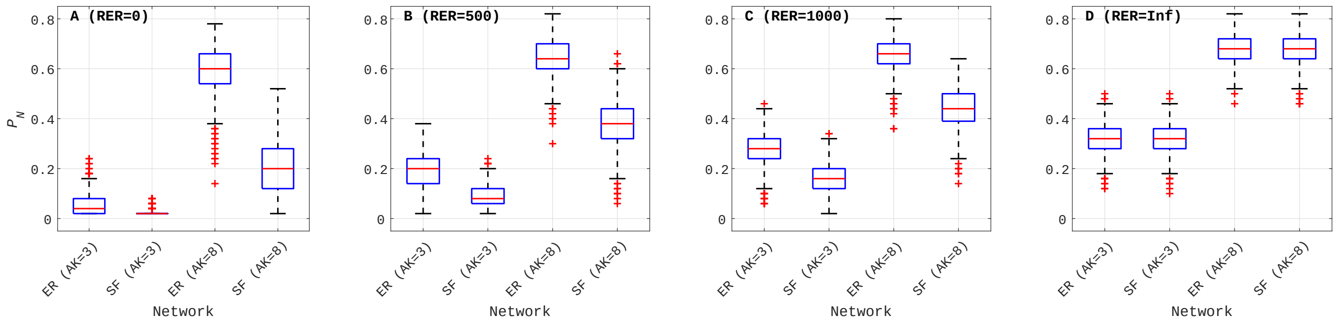


Figure S9: Proportion of random node-removals (denoted by $P_N$) to disconnect a network: (A) without any rectification; (B) with 500 RER operations; (C) with 1000 RER operations; (D) with RER operations until ENC is satisfied.

# 4 Network Size $N = \{500, 2000\}$

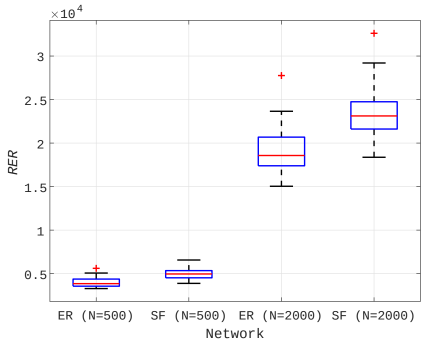


Figure S10: Number of RER operations to rectify a network to satisfy the ENC. The network configuration is $N = 500$ and $N = 2000$; the number of repeated runs is 100.

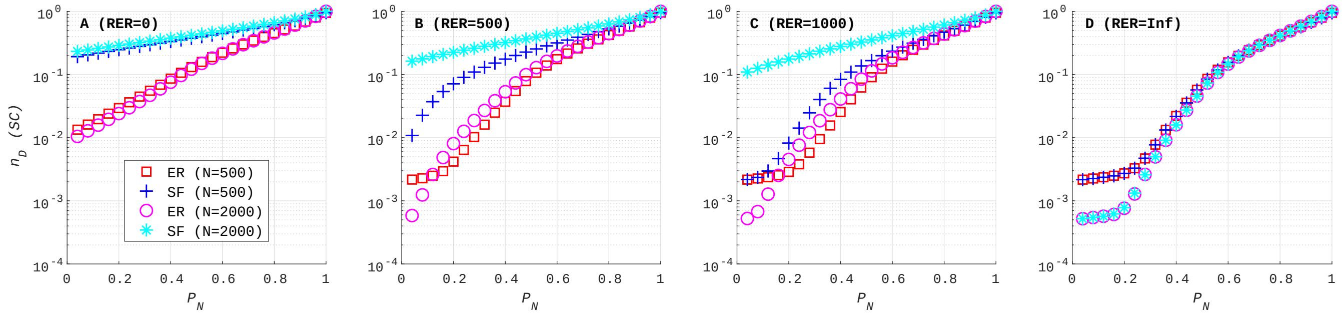


Figure S11: Robustness of *structural* controllability of the six networks: (A) without any rectification; (B) with 500 RER operations; (C) with 1000 RER operations; (D) with RER operations until ENC is satisfied. $n_D$ represents density of control-nodes; $P_N$ represents the proportion of removed nodes.

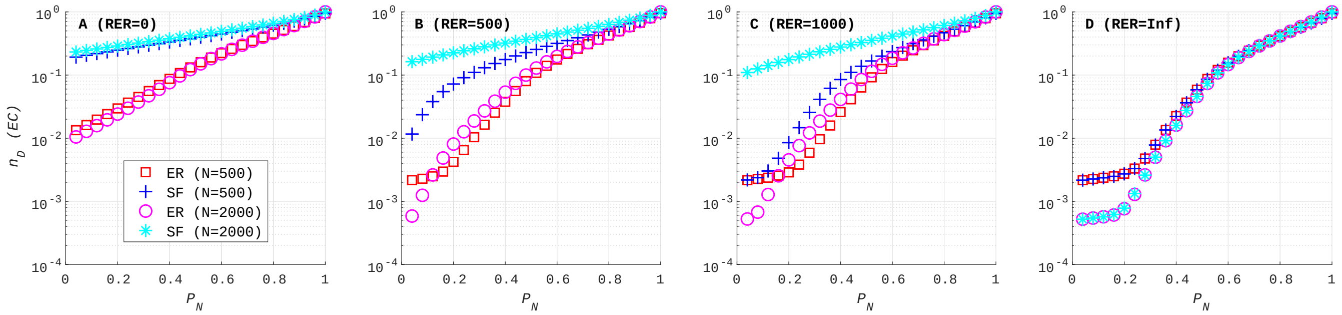


Figure S12: Robustness of *exact* controllability of the six networks: (A) without any rectification; (B) with 500 RER operations; (C) with 1000 RER operations; (D) with RER operations until ENC is satisfied. $n_D$ represents density of control-nodes; $P_N$ represents the proportion of removed nodes.

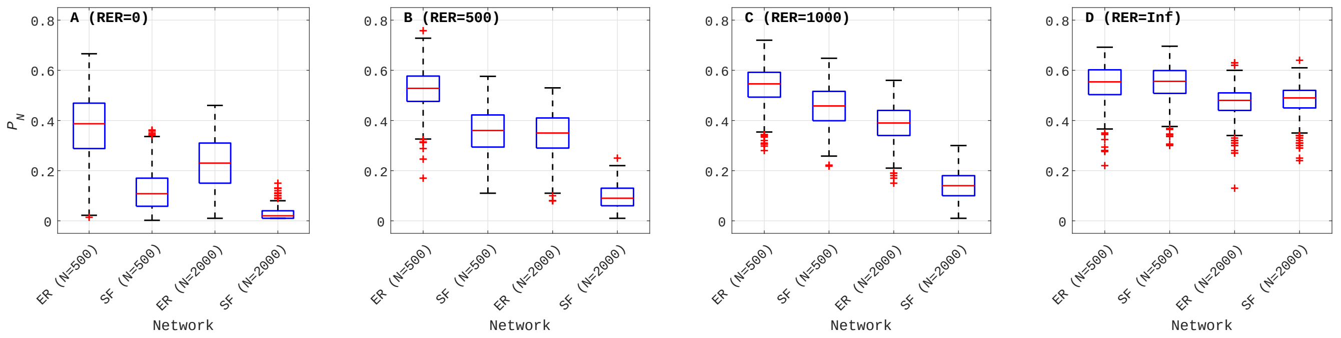


Figure S13: Proportion of random node-removals (denoted by $P_N$) to disconnect a network:(A) without any rectification; (B) with 500 RER operations; (C) with 1000 RER operations; (D) with RER operations until ENC is satisfied.

# 5 Other Supplementary Information

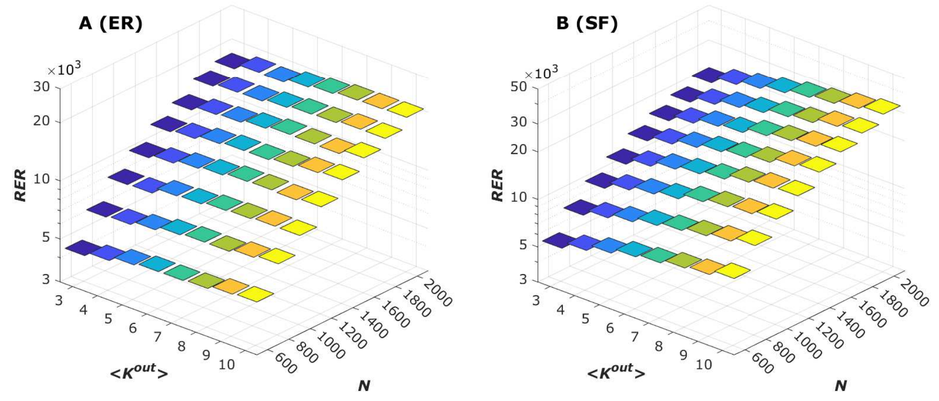


Figure S14: Average number of RER operations to rectify a network to full satisfy the ENC: (A) ER and (B) SF. $\langle k^{out} \rangle$ represents the average out-degree; $N$ represents network size. The number of repeated runs is 100.

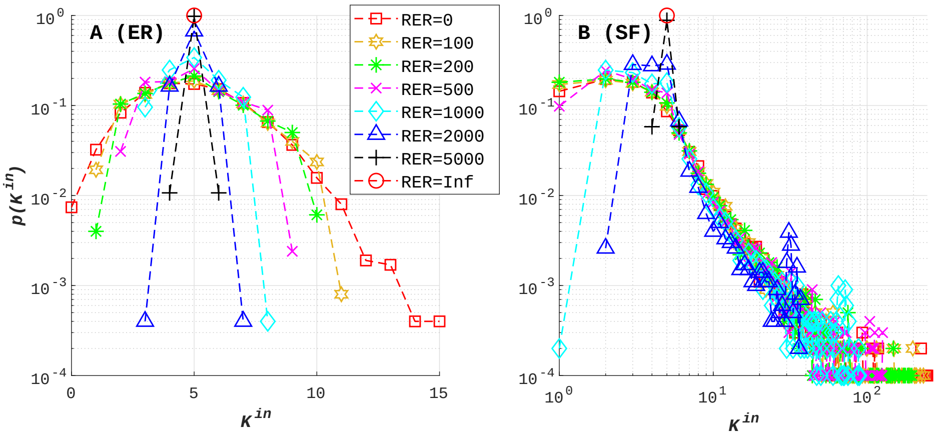


Figure S15: In-degree distribution changes as the number of RER increases: (A) ER and (B) SF.
